# Supplementary material for: Time Adaptive Gaussian Model
Source: arXiv:2102.01238 source file (2021-02-03)
Supplement: Supplementary file 1 [file appendix.tex]

\section{Initialization choices}
The EM algorithm requires an initialization of the parameters $\theta_{old}$. Since the likelihood function we are considering is non-convex the parameters initialization is crucial to find the optimal solution.  In particular,given the cluster number $K$ we have to initialize four parameters: the transition matrix $A$ and the initial probabilities $\+\pi$ and the Gaussian distribution parameters $\+\Theta$ and $\+\mu$.
In our implementation \footnote{\texttt{link-omitted-for-anonimity}} we provide several initializations choices:
\begin{itemize}
    \item \textbf{the transition matrix $A$ and the initial probabilities $\+\pi$} can either be initialised with equal probabilities for each state $\frac{1}{K}$ or by randomly sampling from a uniform distribution  $\mathcal U(0,1)$ or Dirichlet distribution Dir$(1s)$, with the constraints that each row has to sum to one.
    \item \textbf{The Gaussian distribution parameters $\+\Theta$ and $\+\mu$}: we start by computing the  initial subdivision into clusters. In literature the most common way is through the K-means. Since the dependency of the HMMs to Gaussian mixture model (GMM) we also allow the initialization with GMM. Both GMM and K-means are non-convex, thus, depending on initialisation lead to different solutions as well. 
    
    Given the dataset initial subdivision, we compute respectively the empirical covariances and means. Finally we run the graphical lasso to compute the corresponding precision matrix.
\end{itemize}

\section{Model selection}

Our model has two hyper-parameters to cross-validate:
\begin{enumerate}
\item the number of finite states $K$;
\item the regularization parameter $\lambda$ which regulates the sparsity of the precision matrix $\Theta_k$;
\end{enumerate}

To estimate these two hyper-parameters we employ two different kinds of cross validation (CV), Bayesian Information Criterion (BIC) and the Stability of clusters (SoC), when we are cross-validating one hyper-parameter we suppose that the other one is fixed. 
\begin{figure}[t]
    \centering
    \includegraphics[width=0.9\textwidth]{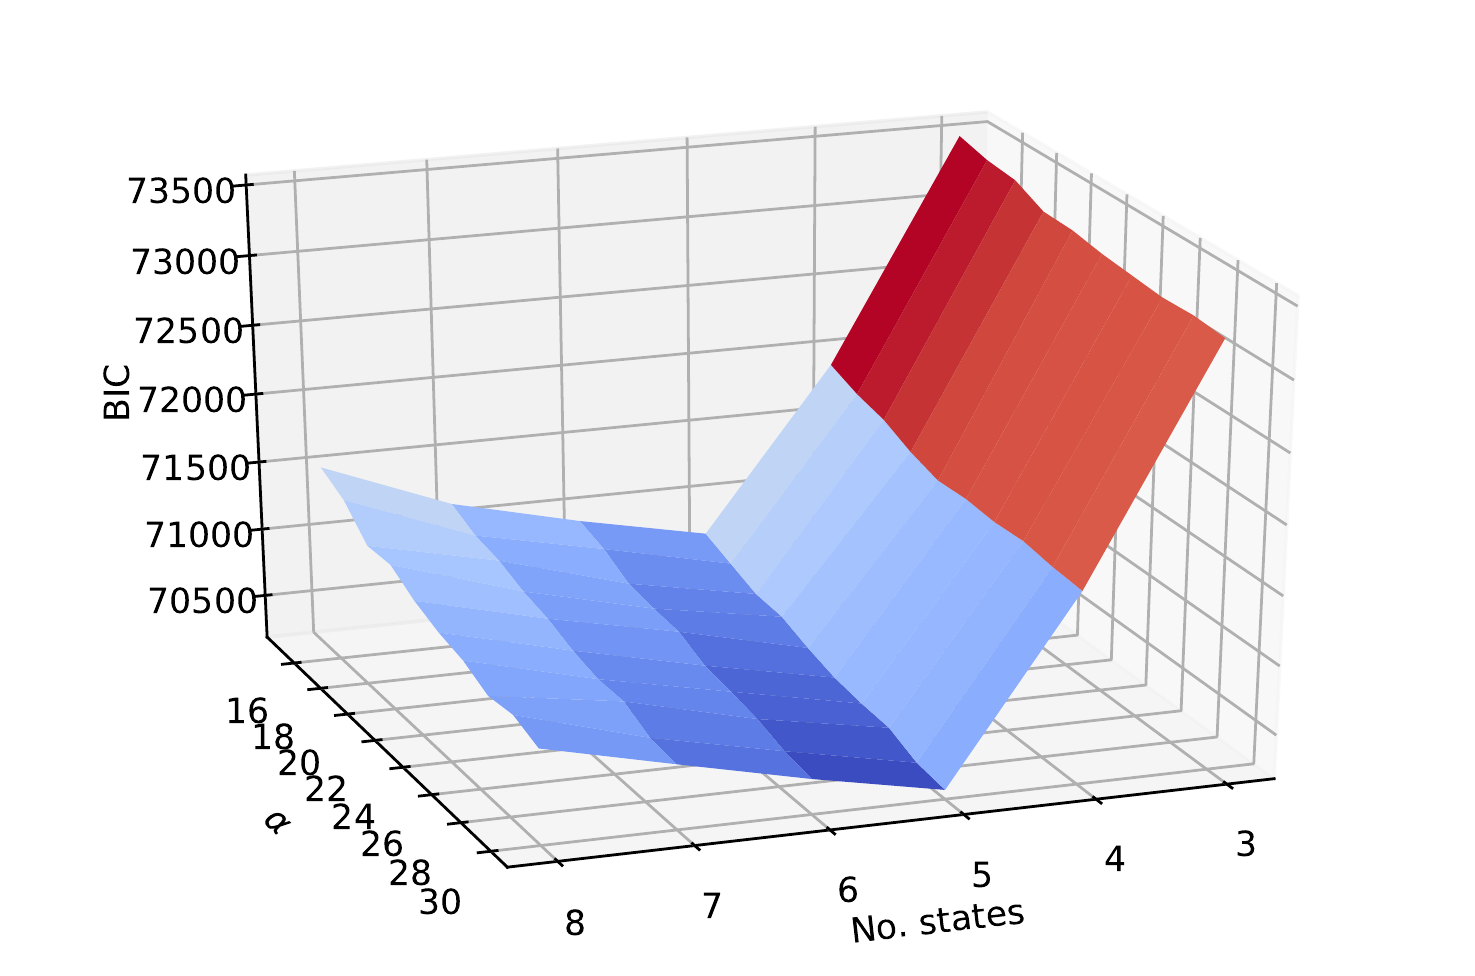}
    \caption{Cross validation}
    \label{CV}
    \end{figure}
Based on our experiments we noticed that the best performances were obtained when we used the BIC to estimate $K$ while the SoC for $\lambda$.
To see that this CV combination of methods is suitable for the estimation of the hyper-parameters of our model we generated a multivariate time series with $d=10$ and $K=5$ and we cross-validate $K$ and $\lambda$ from the sets $K\in\{3,\dots,8\}$ and $\lambda\in$ numpy.linspace$(18,25,10)$. We show in Figure \ref{CV} the results and as we can see it found the $K$ from which we have generated the data.

\subsection{Bayesian Information Criterion (BIC)}
To determine the number of hidden states we use the BIC approach  \cite{schwarz1978} which has the form
\[
\text{BIC}(m)= \ln\+p(\+X|m,\theta)-\frac{\nu}{2}\ln(n).
\]
$\nu$ represents the number of free parameters and  $m$ the considered model. In our case the number of free parameters can be computed in the following:
\begin{itemize}
\item the probabilities $\pi$ have dimension $K$ with one constraint, so $\nu_{\pi}=K-1$;
\item the transition matrix $A$ has dimension  $K\times K$ but each row has a constraint, so $\nu_{A}=K(K-1)$;
\item the means $\mu$ are $K$ with dimension  $d$ without any constraint, so $\nu_{\mu}=Kd$;
\item the precision matrices $\Theta$  are $K$, one for each state, with dimension $d\times d$ but they have the constraint given by graphical lasso therefore $\nu_{\Theta} = \sum_{i\geq j} e_{i,j}$ where $e_{i,j}= 0$ if $\hat{\Theta}_{i,j}=0$  and $e_{i,j}= 1$ otherwise. $\hat{\Theta}$ is the estimated precision matrix.
\end{itemize}
Putting all together the total number of free parameter $\nu$ is 
\[
\nu = \nu_{\pi}+\nu_{A}+\nu_{\mu}+\nu_{\Theta} =(K-1)(K+1)+Kd+\sum_{k=1}^K\nu_{\Theta_k} .
\]

\subsection{Stability of clusters}
The choice of the number of states $K$ can also be performed by looking at the stability of the inferred clusters \cite{brunet2004metagenes}.  Such analysis is reached by fitting the algorithm a certain number of times with different initializations. 
For each repetition we compute the \emph{connectivity matrix}, $C$ \textit{i.e.} a matrix that has $C_{ij} =1$ if the state $i$ and the state $j$ belong to the same cluster and 0 otherwise. 
We then take the mean of the connectivity matrices into a consensus matrix $\bar{C}$ that has in each entry the probability that the states $i$ and $j$ belong to the same cluster. 
On this matrix we can compute the dispersion coefficients that provide us a measurement of how much the clustering is stable \cite{kim2007sparse}.

\section{Synthetic dataset generation}

Real world time-series behaviour have a deep dependence on the sequence in which they appear and the relations among them can change in time. For these reasons we generate synthetic data which are tied together by a Markov process which controls the probability to remain in the same state or to go from one state to another one. To not have a sudden transition from one state to another, we define the variable $S_t$, the \textit{smooth transition} variable, which counts the number of steps necessary to go from state $i$ to state $j$, with $i\not = j$ and $i,j\in \{1,\dots,K\}$.

The synthetic data generation comprehend the following steps:
\begin{enumerate}
    \item we fix suitable values for:
    \begin{enumerate}
        \item \textbf{N}: the number of observations;
        \item \textbf{K}: the number of states;
        \item \textbf{d}: the number of multivariate time series;
    \end{enumerate}
    \item for every state $k\in K$, in our implementation we allow for several combinations of distributions to generate the observations. The idea is to study the behavior of the algorithm in many peculiar cases when the labels are known and from this experience try to interpret the behavior in the real dataset case when the labels are unknown.
    \begin{enumerate}
        \item The mean can be drawn in two ways 
	\begin{enumerate}
		\item if someone wants to generate means which are close to zero like in the stock return case he can pick the \textit{normal 						distribution} case with $\+\mu_k\sim \mathcal{N}(\+0, \mathcal{I}$), where $\mathcal{I}$ is the identity matrix;
		\item otherwise, \textit{uniform distribution} case with $\+\mu_k\sim \mathcal{U}(a,b)$ and $a,b \in \mathbb{R}$ with $a<b$. If $a\ll b$
			then the generated cluster are more likely to be separated between each other.  
	\end{enumerate}
        \item  The covariance matrix $\Sigma_k$ can be set  in three ways: 	
	\begin{enumerate}
        \item generating the precision matrix similarly to what was proposed in \cite{meinshausen2006high,yuan2012discussion}, fixing a certain maximum degree for each node $d$, we randomly selected its neighbours and put deterministically the weights of the edges to $0.98/d$ to ensure positive definiteness of the resulting precision matrix;
    	\item from the tool \textbf{scikit-learn.datasets} which generates a random symmetric, positive-definite matrix; 
		\item from the precision matrix stressing the links between nodes, starting from the identity matrix and putting randomly ones in the off-diagonal places respecting the symmetric matrix constraint. In this way we are generating precision matrix with either strong links between nodes or no links at all. This case is interesting because in this way the networks corresponding to each state $k$ are very different between each others like the case with means very far away.
	\end{enumerate}
    \end{enumerate}
   \item  each row of the transition matrix $A$ is generate from a Dirichlet distribution Dir$(\+\alpha)$ where $\+\alpha\in \mathbb{R}_+^{K}$. In particular, to not have too quick transitions from one state to another we impose $\alpha_i= \kappa\cdot \alpha_j$ with $i\not=j$ where $i$ is the index of the row transition we are drawing and $\alpha_j$ all the other element of $\+\alpha$ different than $\alpha_i$. $\kappa$ is also known  as the \textit{force} constant, in the sense that the bigger $\kappa$ is the more likely the state $i$ is respect to the others;
   \item at each step $n$ the state $k$ is drawn from the transition matrix $A$ then the data are drawn from the normal distribution $\+X_n\sim\mathcal{N}(\+\mu_k,\Sigma_k)$.
\end{enumerate}
From the above description it is possible to note that the introduction of the variable $S_t$ gives the freedom to create different kind of datasets according to their transition between states. Moreover, if we fix $S_t = \Bar{S}_t$  during the transition from state $i$ to state $j$ the data will be drawn from a weighted sum of the parameters which characterise the two states. If during this transition a third state is drawn then the weights will be recalibrated for the three states and so on.

So our datasets will differentiate according to $S_t$ and how we define the transition weights. In particular, we have:

\begin{enumerate}
    \item the \textbf{sudden transition} dataset: where $S_t=1$ fixed and therefore we have no smooth transition;
    \item the \textbf{fixed smooth transition} dataset: where $S_t=\Bar{S}_t\in\mathbb{Z}_+$ always and the weighted sum will take into account how many consecutive steps travelling to the destination we have done so far;
    \item the \textbf{random smooth transition} dataset: where $S_t=\Bar{S}_t\sim \mathcal{U}(a,b)$, with $a,b>1$ and $b>a$. The weights will be set as in 2. but if during a transition another state is drawn then the $\Bar{S}_t$ in this case will replace the previous one and the weights will be recomputed from the latter;
     \item the \textbf{random smooth transition and random weights} dataset: the setting is as in 3. But the weights in this case are drawn randomly from Dir$(\+\alpha)$ with $\+\alpha$ is a vector of $1$s.
\end{enumerate}

\section{Evaluation metrics}
We use a metric score for each of the following aspects:
\begin{enumerate}
\item \textbf{clustering performance}: we compare the clustering results in terms of V-measure \cite{rosenberg2007v} which return a value $v\in[0,1]$ where $v=0$ means that the cluster labels are assigned completely randomly while $v=1$ means that there is a perfect match between the true labels and the one found by the models. 
\item \textbf{network inference performance}: in order to evaluate the performances of the methods we need to identify a map between the true clusters and the identified ones in order to compare the underlying graphs. Such map is obtained by taking the maximum per row of the contingency table of the true and predicted labels. 
We then consider the true and inferred graphs as binary classes (0 no edge identified, 1 edge identified) and we compute the Matthews correlation coefficient (MCC) \cite{matthews1975comparison} which return a value in the interval$[-1,1]$ where $0$ corresponds to chance.
\item \textbf{forecasting performance}: we used as score the Mean Absolute Error (MAE) which measures the error between the true next point value and the predicted one. Since we are predicting $d$ values for each future time point we compute the mean MAE across entries of the vector: $$
MAE = \frac1n\sum_{i=1}^N \bigg(\frac1d\sum_{j=1}^d |x_{nj} - \hat{x}_{nj} |\bigg)
$$.
\end{enumerate}

\section{Higher order extension: Memory Time Adaptive Gaussian model (MemTAGM)}
Sometimes real world applications have events which rely on their past realizations. Therefore we can exploit more information from data if we consider a higher-order Markov process whose $\+z_n$ state probability does not depend only on $\+z_{n-1}$ but also on the other $r$ past states according to the choice of $r$. TAGM can be extended to higher order sequential relationships. We consider a homogeneous Markov process of order $r\in\mathbb{Z}^+$ over a finite state set $\{1,\dots,K\}$ with hidden sequence $\{\+z\}_{n=1}^N$. This stochastic process satisfies 
\[
p(\+z_n|\{\+z_\ell\}_{\ell<n})=p(\+z_n|\{\+z_\ell\}_{\ell=n-r}^{n-1})
\]
or in other words $\+z_n$ can depend on a different number of hidden past states, and we assume that the process is homogeneous i.e., the transition probability 
%$p(\+z_n|\{\+z_\ell\}_{\ell=n-r}^{n-1})$ 
is independent of $n$. To be as more general as possible we allow that the emission probability of $\+x_n$ can depend not only on $\+z_n$ but also from the previous $m\in\mathbb{Z}^+$ sequence of states
\[
p(\+x_n|\{\+x_\ell\}_{\ell<n},\{\+z_\ell\}_{\ell\leq n})= p(\+x_n|\{\+z_\ell\}_{\ell =n-(m-1)}^n).
\]
Each observation is conditionally independent of the previous ones and of the state sequence history, given the current and the preceding $m-1$ states.

The idea is transform the High order hidden Markov model (HHMM) to a first order hidden Markov model (HMM). It can be done by considering the following two propositions where we omit the prove but it can be found in  \cite{hadar2009high} 
\begin{proposition}
Let $\+Z_n = [\+z_n,\+z_{n-1},\dots,\+z_{n-(\nu-1)}]^\top$. The process $\{\+Z_n\}$ is a first order homogeneous Markov process for any $\nu\geq r$, taking values in $\mathcal{S}^\nu$.
\end{proposition}
\begin{proposition}\label{prop2}
Let $\nu= \max\{ r,m\}$. The state sequence $\{ \+Z_n\}$ and the observation sequence $\{ \+x_n\} $ satisfy
\[
p(\+x_n|\{\+x_\ell\}_{\ell<n},\{\+z_\ell\}_{\ell\leq n})= p(\+x_n|\+Z_n)
\]
and thus constitute a first order  HMM.
\end{proposition}

We can  thus reformulate HHMM as a first order HMM with $K^\nu$ states, where $\nu = \max\{r,m\}$. 
Note that the last $\nu-1$ entries of $\+Z_n$ are equal to the first $\nu-1$ entries of $\+Z_{n+1}$, one concludes that a transition from $\+z_n$ to $\+z_{n+1}$ is possible only if $\lfloor \+z_n/K\rfloor=\+z_{n+1}-\lfloor \+z_{n+1}/K^{\nu-1}\rfloor K^{\nu-1}$, and thus
\[
A_{i,j}=0\quad\text{if }\Big\lfloor \frac{i}{K}\Big\rfloor\not = j-\Big\lfloor \frac{1}{K^{\nu-1}}\Big\rfloor K^{\nu-1}.
\]
Therefore we can use the EM algorithm to find the optimal parameters changing the number of states to $K^\nu$. The $z_{n,j}$s which contribute to the M step for a quantity of state $i$ are given by the set
\[
\mathcal{I}_m(i)=\Bigg\{\Big\lfloor\frac{i}{K^{\nu-m}}\Big\rfloor K^{\nu-m},\Big\lfloor\frac{i}{K^{\nu-m}}\Big\rfloor K^{\nu-m}+1,\dots,\Big(\Big\lfloor\frac{i}{K^{\nu-m}}\Big\rfloor +1\Big)K^{\nu-m}-1\Bigg\}.
\]
Therefore the means become
\[
\mu_i=\frac{\sum_{n=1}^N\+x_n\sum_{j\in\mathcal{I}_m(i)}\gamma(z_{n,j})}{\sum_{n=1}^N\sum_{j\in\mathcal{I}_m(i)}\gamma(z_{n,j})}
\]
The empirical covariances to substitute in the graphical lasso equation is
\[
\Tilde{S}_i= \frac{\sum_{n=1}^N(\+x_{n}-\+\mu_i)(\+x_{n}-\+\mu_i)^\top\sum_{j\in\mathcal{I}_m(i)}\gamma(z_{n,j})}{\sum_{n=1}^N\sum_{j\in\mathcal{I}_m(i)}\gamma(z_{n,j})},
\]
with the hyper-parameter $\tilde{\lambda}_k=\frac{\lambda}{\sum_{n=1}^N\sum_{j\in\mathcal{I}_m(i)}\gamma(z_{n,j})}$. The transition probability matrix becomes
\[
A_{i,j}=
\begin{cases}
&\frac{\sum_{n=2}^N\sum_{k\in\mathcal{I}_r(i)}\xi(z_{n-1,k},z_{n,\lfloor\frac{k}{K}\rfloor+\lfloor\frac{j}{K^{\nu-1}}\rfloor K^{\nu-1}})}{ \sum_{l=1}^{K^\nu}\sum_{n=2}^N\sum_{k\in\mathcal{I}_r(i)}\xi(z_{n-1,k},z_{n,l})}\quad\text{if }\lfloor\frac{i}{K}\rfloor=j-\lfloor\frac{j}{K^{\nu-1}}\rfloor K^{\nu-1},\\
&0\quad\text{otherwise}.
\end{cases}
\]
Finally,  the initial state probabilities are given by
\[
\pi_i=\gamma(z_{1,i}).
\]
Therefore if we increase the number of states to $K^{\nu}$ and modify the TAGM M step formulas with the one just found we obtain the MemTAGM. We test MemTAGM performance in subsection 9.2 where we compare it with TAGM.

\section{On-line learning: Incremental Time Adaptive Gaussian model (IncTAGM)}
In many applications it is important to update the TAGM parameters almost instantaneously every time a new observation comes up. Since TAGM does not allow to have such a quick response, it can be extended to an incremental version. We call this model IncTAGM and it initially starts as a standard TAGM reading a set of observations and updating its current parameters $\pi,A, \mu, \+\Theta$ according to new incoming data. Therefore, after the standard TAGM has finished training on its observation set, it calculates the revised $\alpha, \beta, \xi$ and $\gamma$ variables based on the new set of observations. To update the model incrementally, we need recursive equations for $\alpha$ and $\beta$ which depend on past values. Notice that the $\alpha$ recursive equation is already of this form. While the $\beta$ recursive equation needs an approximation to become of that form. In fact if we assume that $\beta(z_{T,i})\simeq \beta(z_{T,j})$ for every $i\not=j$, the $\beta$ recursive equation becomes
\begin{equation}
\beta(\+z_{T+1}) =\frac{\beta(\+z_{T}) }{\sum_{\+z_{T+1}}p(\+x_{T+1}|\+z_{T+1})p(\+z_{T+1}|\+z_T)}.
\end{equation}

The M step optimal parameters are updated in the following way:

the initial state $\pi$
\begin{equation}
\pi_k' =\gamma(z_{1,k}),
\end{equation}
the transition matrix $\+A$ 
\begin{align}
A^{T+1}_{j,k} &= \frac{ \sum_{n=2}^T\xi(z_{n-1,j},z_{n,k})+\xi(z_{T,j},z_{T+1,k})}{\sum_{l=1}^K\sum_{n=2}^T\xi(z_{n-1,j},z_{n,l})+\sum_{l=1}^K\xi(z_{T,j},z_{T+1,l})}\notag\\
&= \frac{ \sum_{n=2}^T\xi(z_{n-1,j},z_{n,k})}{\sum_{n=2}^{T+1}\gamma(z_{n-1,j})} + \frac{\xi(z_{T,j},z_{T+1,k})}{\sum_{n=2}^{T+1}\gamma(z_{n-1,j})}\notag\\
&= \frac{ \sum_{n=2}^{T}\gamma(z_{n-1,j})}{\sum_{n=2}^{T+1}\gamma(z_{n-1,j})} \frac{ \sum_{n=2}^T\xi(z_{n-1,j},z_{n,k})}{\sum_{n=2}^{T}\gamma(z_{n-1,j})}  + \frac{\xi(z_{T,j},z_{T+1,k})}{\sum_{n=2}^{T+1}\gamma(z_{n-1,j})}\notag\\
&= \frac{ \sum_{n=2}^{T}\gamma(z_{n-1,j})}{\sum_{n=2}^{T+1}\gamma(z_{n-1,j})}A^{T}_{j,k} + \frac{\xi(z_{T,j},z_{T+1,k})}{\sum_{n=2}^{T+1}\gamma(z_{n-1,j})}.\label{recA}
\end{align}
Note that if we sum by $k\in\{1,\dots,K\}$ the row normalization holds. Similarly we obtain the formula for the means
\begin{equation}
\mu_k^{T+1}=\frac{ \sum_{n=1}^{T}\gamma(z_{n,k})}{\sum_{n=1}^{T+1}\gamma(z_{n,k})}\mu_k^T+\frac{\gamma(z_{T+1,k})\+x_{T+1}}{\sum_{n=1}^{T+1}\gamma(z_{n,k})}
\end{equation}
and the empirical covariances
\begin{equation}
\Tilde{S}^{T+1}_k=\frac{ \sum_{n=1}^{T}\gamma(z_{n,k})}{\sum_{n=1}^{T+1}\gamma(z_{n,k})}\Tilde{S}^{T}_k+ \frac{\gamma(z_{T+1,k})(\+x_{T+1}-\+\mu^{T+1})(\+x_{T+1}-\+\mu^{T+1})^\top}{\sum_{n=1}^{T+1}\gamma(z_{n,k})},
\end{equation}
 with the hyper-parameter $\tilde{\lambda}_k=\frac{\lambda}{\sum_{n=1}^{T+1}\gamma(z_{n,k})}$.
We test IncTAGM performance in subsection 9.2 where we compare it with TAGM.
\subsection{Slide Incremental Time Adaptive Gaussian model (S-IncTAGM)}
The training of new data points results in the accumulation of an increasingly large observation set. As a result, if the time sequence considered is large and the first point is far away in the past respect to the last point it is possible that the initial trained observation points become outdated after many updates and therefore they do not carry any useful information to analyze the more recent points.  Therefore, the new addition to the IncTAGM is a fixed sliding window to effectively analyze discrete data (appropriately discarding the outdated observations) whilst updating its model parameters. 

The estimation of the $\alpha, \beta, \xi$ and $\gamma$ variables remains the same as in the IncTAGM algorithm. What changes are the $A$, $\+\mu$ and $\+\Theta$ updates. Using the \textit{simple moving average} (SMA) definition
\begin{equation}
sma=\frac{x_1+x_2\dots+x_n+x_{n+1}-x_1}{n}= ave +\frac{x_{n+1}}{n}-\frac{x_1}{n}
\end{equation}
where $ave= \frac{x_1+x_2\dots+x_n}{n}$,  we update $A$, $\+\mu$ and $\+\Theta$ in the following way
\begin{align}
A^{T+1}_{j,k} &= \frac{\sum_{n=3}^{T+1}\xi(z_{n-1,j},z_{n,k})}{\sum_{n=3}^{T+1}\gamma(z_{n-1,j})},\\
\mu_k^{T+1} &=\frac{ \sum_{n=2}^{T+1}\gamma(z_{n,k})\+x_n}{\sum_{n=2}^{T+1}\gamma(z_{n,k})},\\
\Tilde{S}^{T+1}_k&=\frac{ \sum_{n=2}^{T+1}\gamma(z_{n,k})(\+x_{n}-\+\mu^{T+1})(\+x_{n}-\+\mu^{T+1})^\top}{\sum_{n=2}^{T+1}\gamma(z_{n,k})}
\end{align}
with $\tilde{\lambda}_k=\frac{\lambda}{\sum_{n=2}^{T+1}\gamma(z_{n,k})}$.

\subsection{Higher order and on-line extension experiments}
\begin{figure}[t]
    \includegraphics[width=0.5\textwidth]{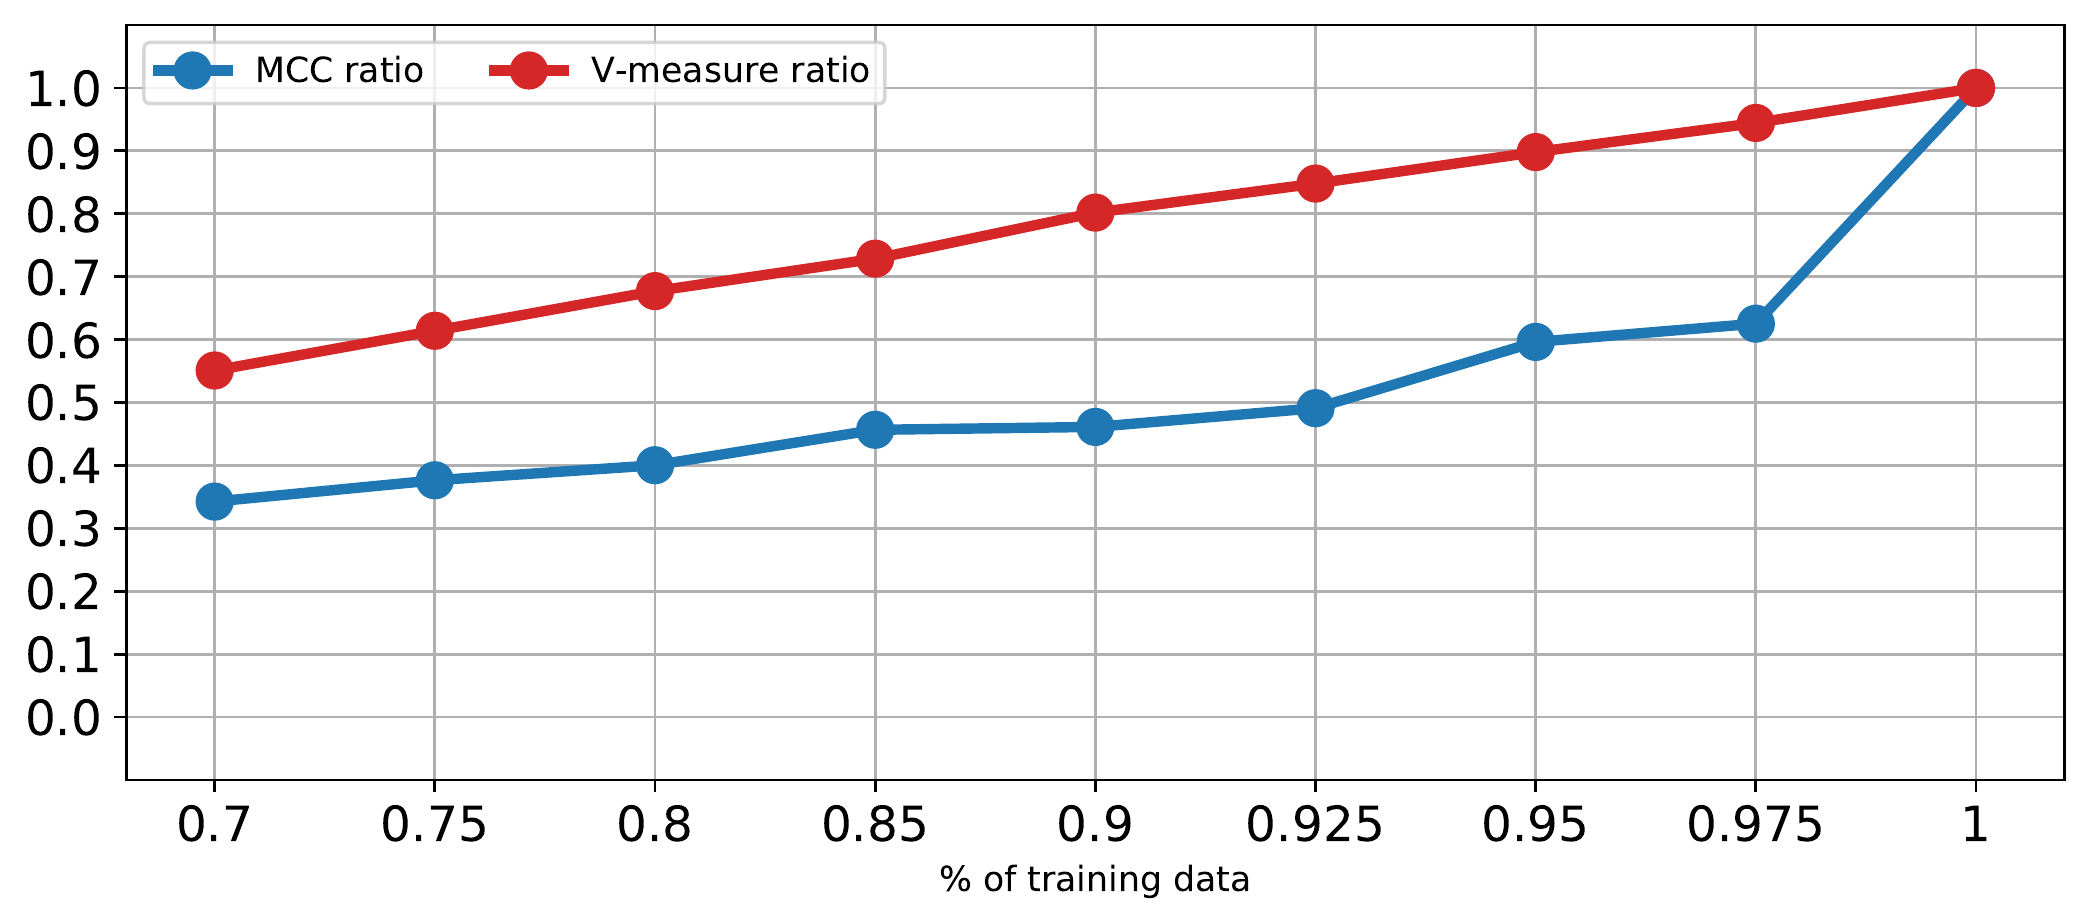} \includegraphics[width=0.5\textwidth]{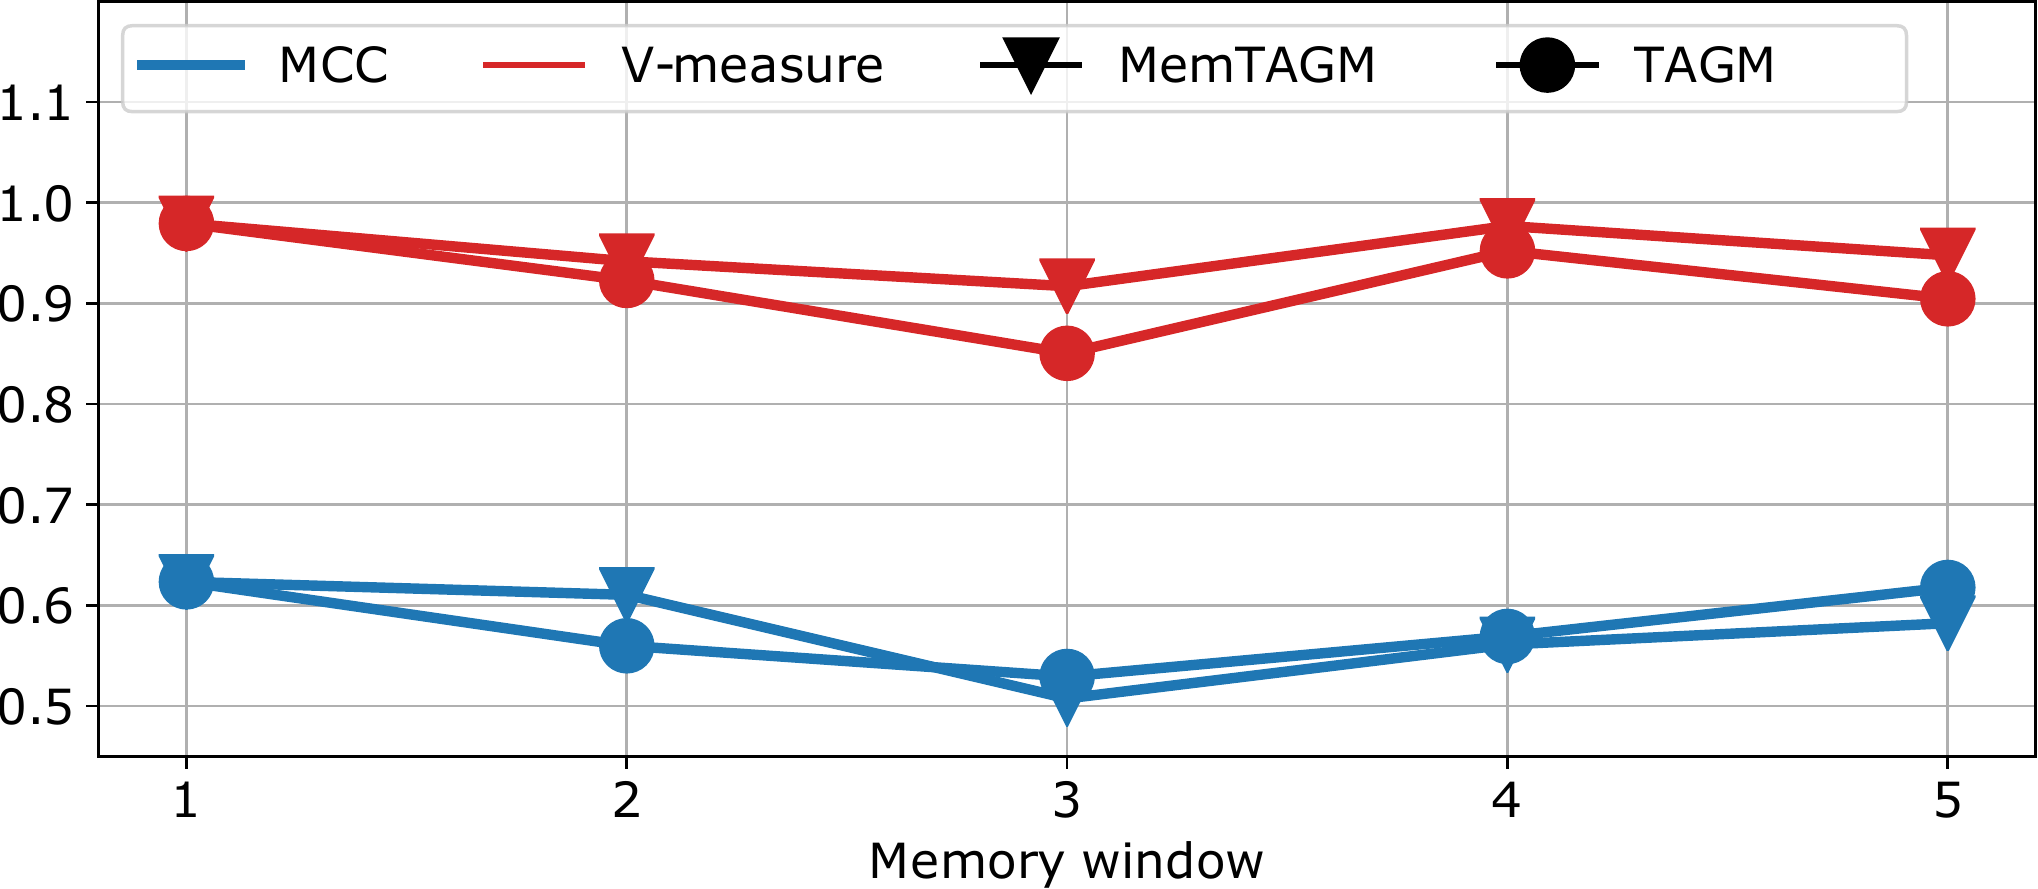}
    \caption{Comparison of TAGM with its extensions in terms of V-measure and MCC. On the left hand panel we drew the  V-measure and MCC ratio of  IncTAGM and TAGM as the number of batch training data increases. On the right hand panel we drew the  V-measure and MCC of  MemTAGM and TAGM as the memory of the hidden Markov process increases. }
    \label{fig:incremental}
    \end{figure}
Using the same setting to generate synthetic data as in section 5 of the main document, we perform two types of experiments to compare the higher order and the incremental extensions with the batch model described in the main document.
\paragraph{TAGM vs IncTAGM:}For this experiment we generated a synthetic dataset with $K=5$ states,  $d=10$ dimensions and $N=2000$ observations. We want to assess the behaviour of IncTAGM w.r.t. TAGM as the percentage of initial data given in input $\hat{N} = \%N$ to IncTAGM increases. The results are shown on the left panel of Figure~\ref{fig:incremental}, where we can see that IncTAGM asymptotically tends to the performance of TAGM as the percentages of input data reaches 100\% but the on-line model performance decreases very quickly when we increase the number of data which make the parameters update on-line.
\paragraph{TAGM vs MemTAGM} For this experiment we generated a synthetic dataset with $K=3$ states,  $d=10$ dimensions and $N=2000$ observations. But, in this case we let the memory of the hidden Markov process vary. In this way we are able to evaluate the behaviour of MemTAGM
w.r.t. TAGM as the memory of the hidden Markov process increases. The results are shown on the right panel of Figure~\ref{fig:incremental}, where we can see that MemTAGM performance in terms of V-measure and MCC is slightly better respect to the one of TAGM as the hidden Markov process memory increases. Recall that the time complexity of the forward-backward algorithm is $O(K^2N)$ and therefore since MemTAGM number of states is $K^\nu$ where $\nu$ is the Markov process memory, the performance improvement does not justify the amount of time needed to wait.
